# Supplementary material for: HAO: Hardware-aware neural Architecture Optimization for Efficient Inference
Source: arXiv:2104.12766 source file (2021-04-26)
Supplement: Supplementary file 1 [file 7_appendix.tex]

\section{Appendix}
Here, we provide additional experimental results as well as quantization
details for the neural networks that we tested.

\begin{itemize}

    \item In~\S~\ref{sec:details} we discuss the fine-tuning details.
    \item In~\S~\ref{sec:extra_results} we present extra results
    for 3D plots for loss landscape of different blocks of ResNet20 and Inception-V3 as well
    as exemplary results showing distribution of $\Omega_i$ in~\eref{eqn:define_O}.

    \item In~\S~\ref{sec:mixed_precision_detail} we show the exact bit-precision used for different
    blocks of ResNet20 on Cifar-10 as well as Inception-V3 on ImageNet.

\end{itemize}

\subsection{Fine-tuning details}
\label{sec:details}
 The results were tested on two classification datasets of Cifar-10 and ImageNet:

\paragraph{Cifar-10} This is a classification dataset with 10 classes
consisting of 50,000 training images and 10,000 test images
 of size $3\times32\times32$.
We used pre-trained ResNet20 model and performed quantization on this
model in PyTorch framework.
We follow the same learning rate policy as the baseline (\emph{i.e.}, decaying learning rate from 
1e-1 to 1e-4).

\paragraph{ImageNet} This is a classification problem with 1000 classes consisting of more than 1.2 million training images 
and 50,000 validation images of size $3\times224\times224$ on SqueezeNext and ResNet50 , and $3\times299\times299$ on Inception-V3.
(i) We used pre-trained Inception-V3 model and used a fixed learning rate of 2e-4 for fine-tuning of each block.
(ii) We used pre-trained ResNet50 model and used a fixed learning rate of 1e-4 for fine-tuning of each block.
(iii) We used pre-trained SqueezeNext and used a fixed learning rate of 1e-4 for fine-tuning of each block.
All experiments were performed on PyTorch framework. As for data augmentation, we used standard random crop, resizing and horizontal flip in all experiments.

\subsection{Extra results}
\label{sec:extra_results}

In~\tref{tab:shift_table}, we show how $\Omega_i$ changes as a function of quantization precision. In~\fref{fig:resnet20_surface_appendix}, we plot the rest surface visualization of ResNet20 on Cifar-10. And in~\fref{fig:inception_surface_appendix}, we plot the rest surface visualization of Inception-V3 on ImageNet.

\begin{table}[!htbp]
\caption{Here we show how $\Omega_i$ changes as a function of 
target weight bit precision. Results are computed for ResNet20
on Cifar-10.}
\vspace{2mm}
\label{tab:shift_table}
\centering
\begin{tabular}{lcccccccccccccc} \toprule
\diagbox[dir=SE]{Block}{Precision} & 8-bit & 6-bit & 4-bit & 3-bit & 2-bit\\
    \midrule
\ha  Block 3    & 0.03 & 0.52 & 9.25 & 41.9 & 191 \\
\ha  Block 5    & 0.05 & 0.81 & 14.0 & 65.1 & 309 \\
\ha  Block 8    & 0.29 & 4.83 & 84.8 & 392  & 2056 \\
     \bottomrule 
\end{tabular}
\end{table}

\begin{figure*}[!htbp]
\centering
\includegraphics[width=.99\textwidth]{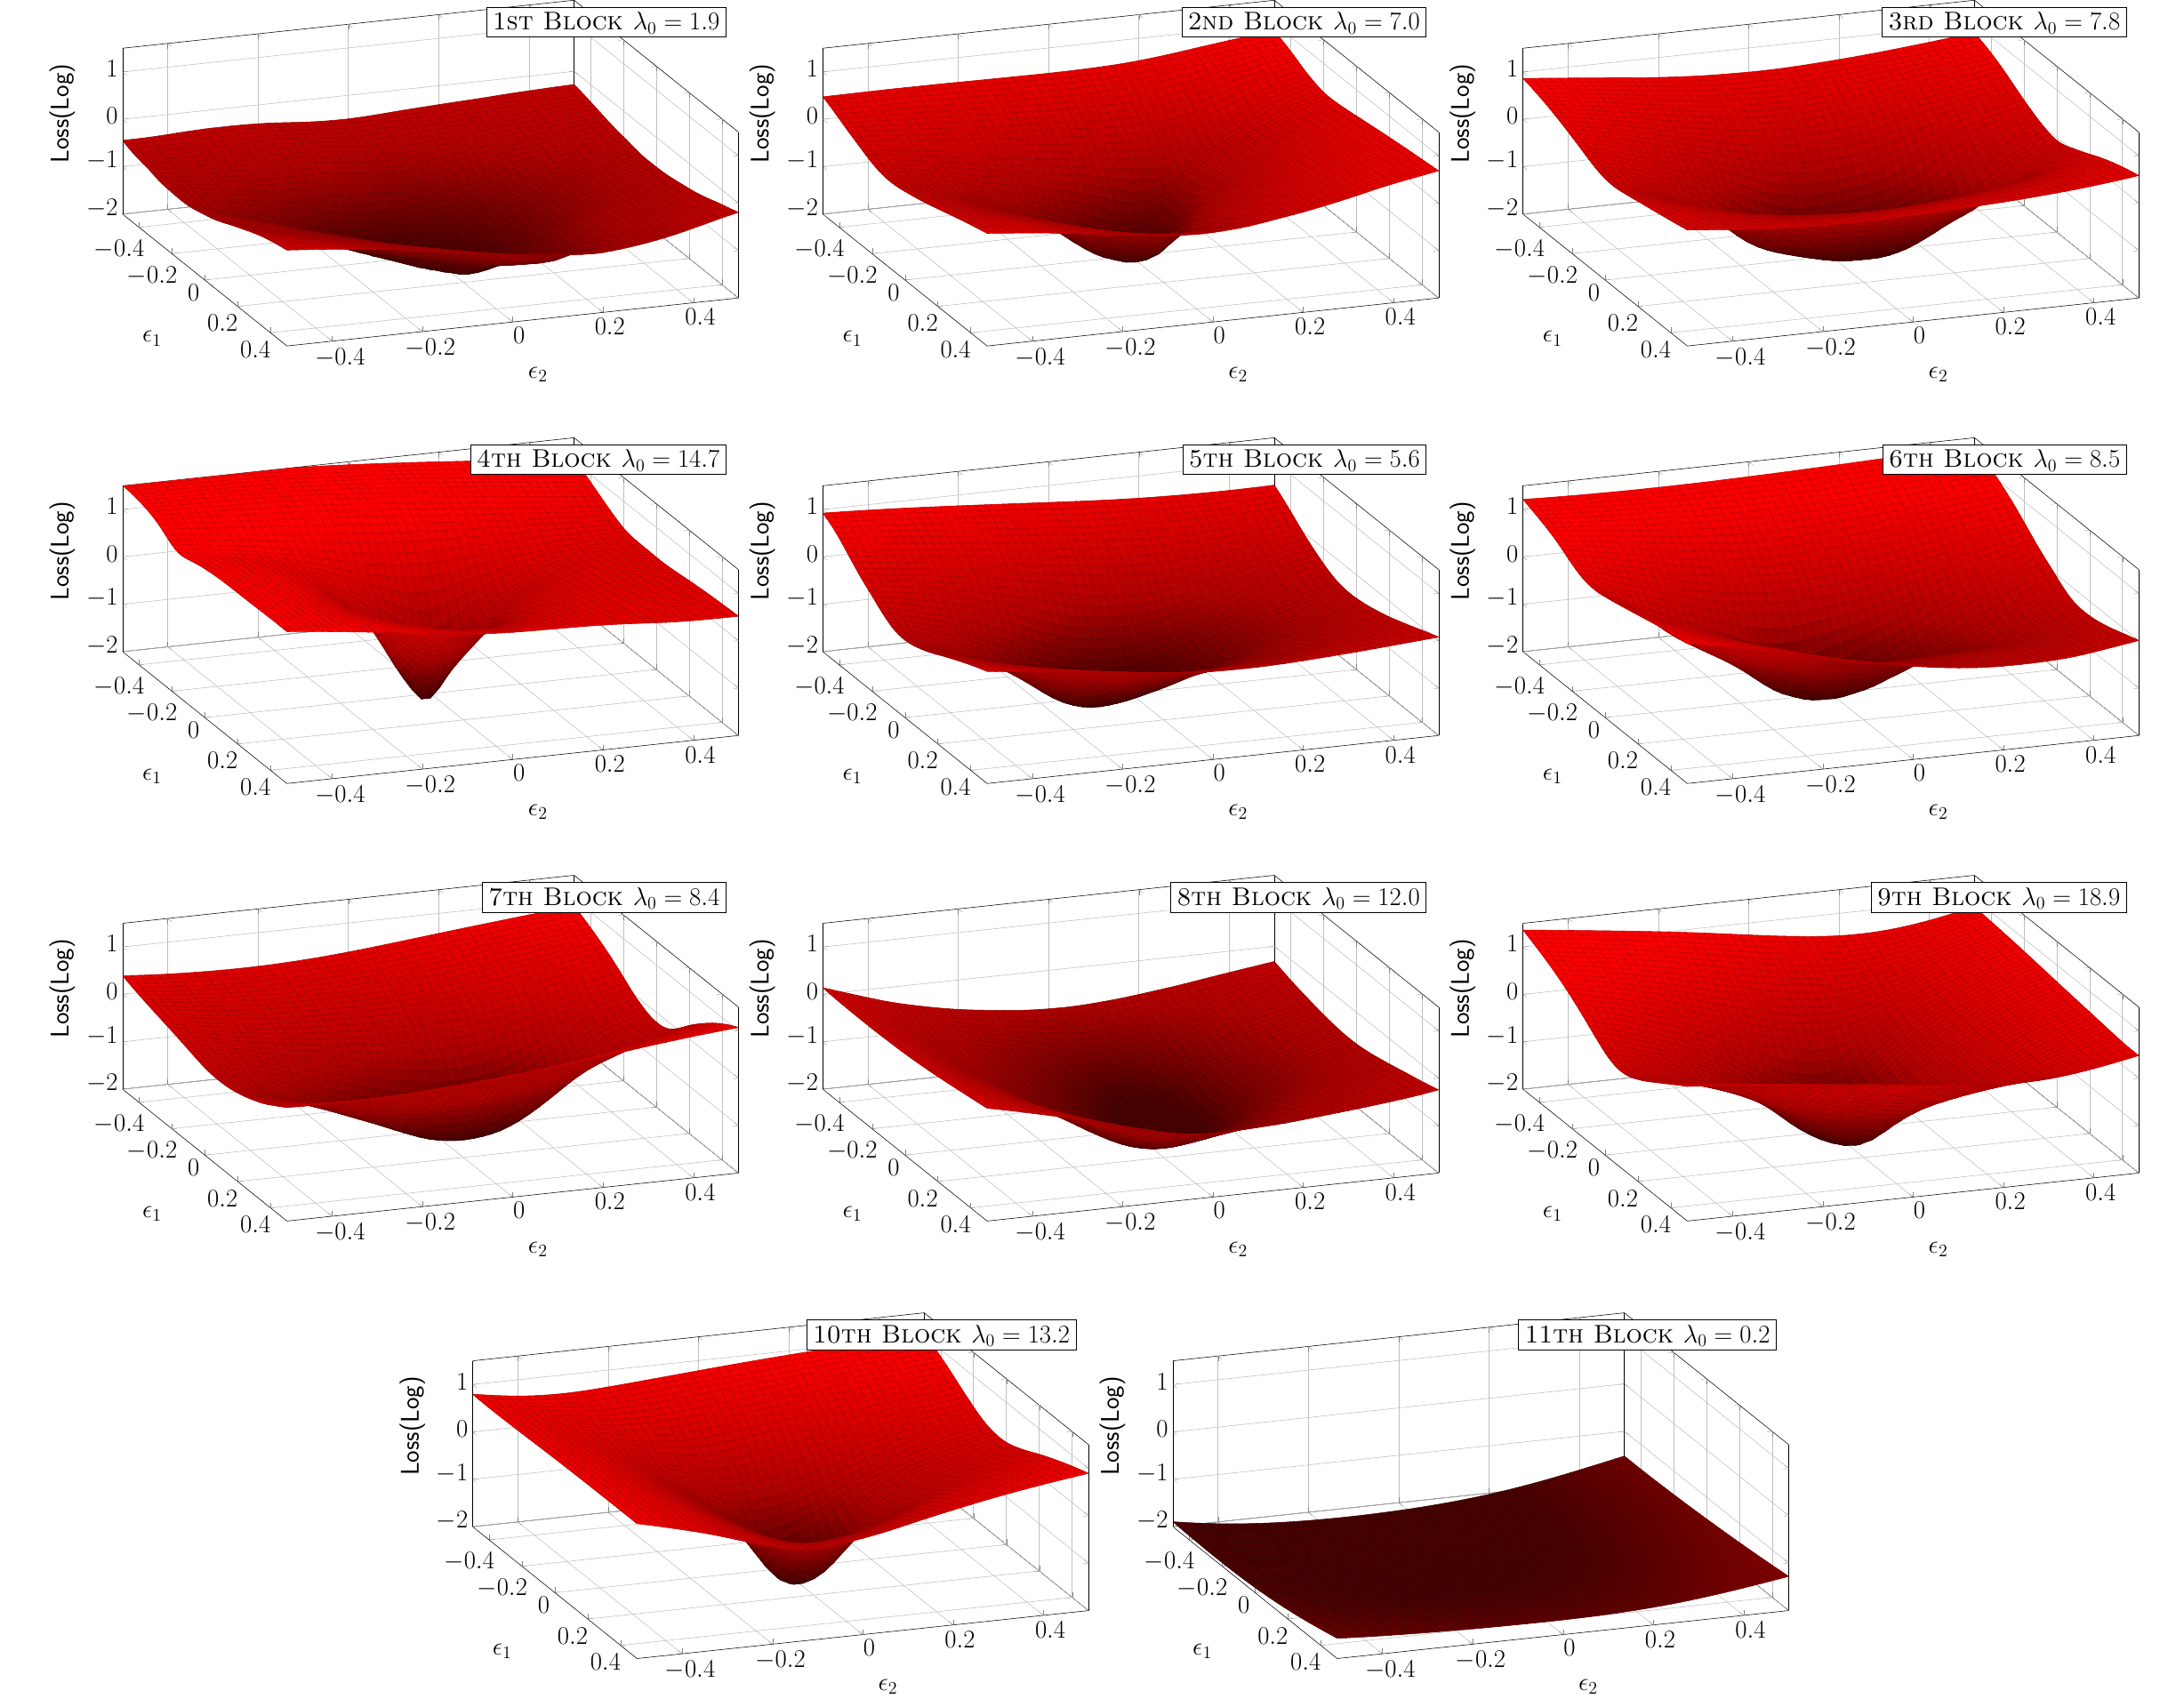}
\caption{
  3-D loss landscape of all blocks of ResNet20 on Cifar-10 along the first two dominant eigenvectors of the Hessian. Here $\epsilon_1$, $\epsilon_2$ are scalars that perturb the parameters of the corresponding block along the first and second dominant eigenvectors. 
  The corresponding eigenvalue distribution for different blocks is also shown in~\fref{fig:resnet_inception_eigs_surface}.
  }
\label{fig:resnet20_surface_appendix}
\end{figure*}

\begin{figure*}[!htbp]
\centering
\includegraphics[width=.99\textwidth]{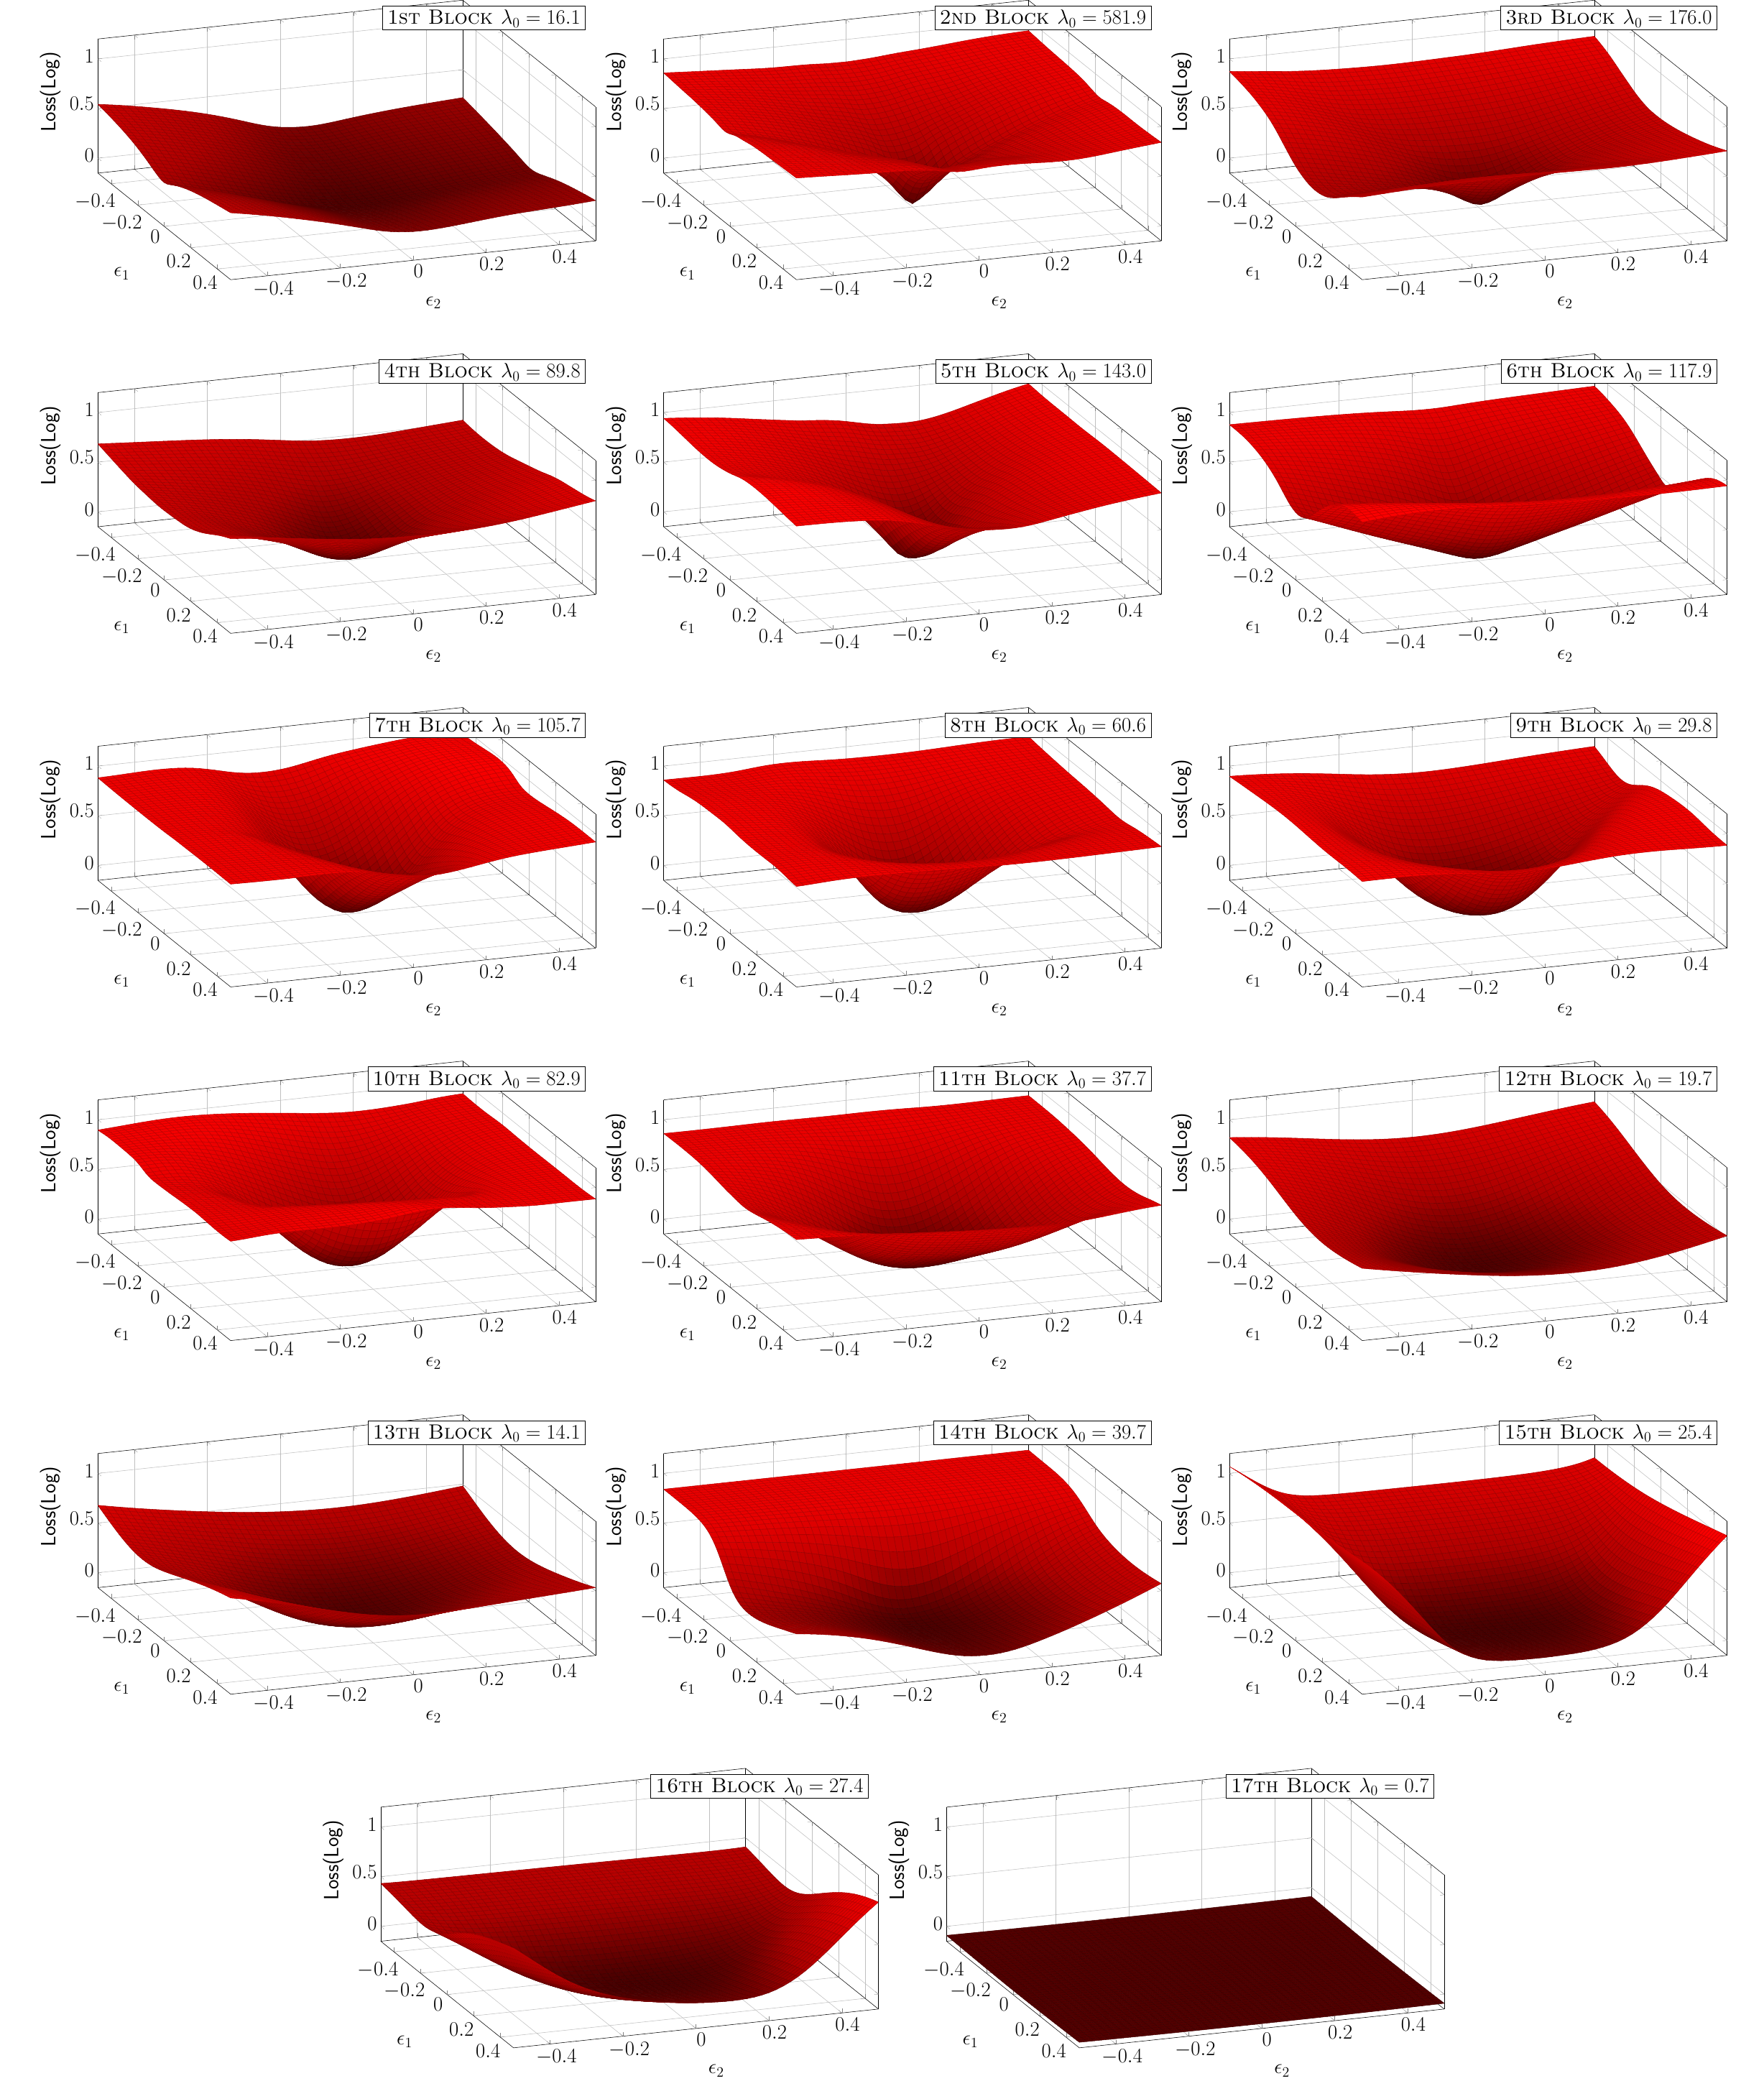}
\caption{
  3-D loss landscape of all blocks of InceptionV3 on ImageNet along the first two dominant eigenvectors of the Hessian. Here $\epsilon_1$, $\epsilon_2$ are scalars that perturb the parameters of the corresponding block along the first and second dominant eigenvectors. The corresponding eigenvalue distribution for different blocks is also shown in~\fref{fig:resnet_inception_eigs_surface}.
  }
\label{fig:inception_surface_appendix}
\end{figure*}

\subsection{Mixed-precision details}
\label{sec:mixed_precision_detail}
In this section, we give the details about how we separate blocks and details about weight/activation precision of each individual block. We show the exact bit-precision used for different
    blocks of ResNet20 (\tref{tab:resnet20_final_precision}) on Cifar-10 as well as Inception-V3 (\tref{tab:inception_final_precision}) on ImageNet.

\begin{table}[!htbp]
\caption{Block seperation and final block precision of ResNet20 on Cifar-10. Here we abbreviate convolutional layer as ``Conv,'' fully connected layer as ``FC.''}
\small
\vspace{2mm}
\label{tab:resnet20_final_precision}
\centering
\begin{tabular}{lcccccccccccccc} \toprule
             &Block     &Layer(s)      &Layer Type    &Parameter Size  & Weight bit & Activation bit
             \\
    \midrule
             & Block 0  & Layer 0     & Conv          &      4.32e2     & 8          & 8 \\
    \midrule
\gc\gc             & Block 1  & Layer 1-2   & Conv          &      4.61e3     & 6           & 4  \\
    \midrule
             & Block 2  & Layer 3-4   & Conv          &      4.61e3     & 6           & 4  \\
    \midrule
\gc\gc             & Block 3  & Layer 5-6   & Conv          &      4.61e3     & 8           & 4  \\
             
    \midrule
             & Block 4  & Layer 7-8   & Conv          &      1.38e4     & 3           & 4   \\
             
    \midrule
\gc\gc             & Block 5  & Layer 9-10  & Conv          &      1.84e4     & 3          & 4   \\
             
    \midrule
             & Block 6  & Layer 11-12 & Conv          &      1.84e4     & 3          & 4   \\
             
    \midrule
\gc\gc             & Block 7  & Layer 13-14 & Conv          &      5.53e4     & 2         & 4   \\
             
    \midrule
             & Block 8  & Layer 15-16 & Conv          &      7.37e4     & 2          & 4   \\
             
    \midrule
\gc\gc             & Block 9  & Layer 17-18 & Conv          &      7.37e4     & 2         & 4   \\
             
    \midrule
             & Block 10 & Layer 19    & FC            &      6.40e2     & 3        & 8 \\
     \bottomrule 
\end{tabular}
\end{table}

\begin{table}[!htbp]
\caption{Block seperation and final block precision of  Inception-V3 on ImageNet. Here we abbreviate convolutional layer as ``Conv,'' fully connected layer as ``FC.''}
\small
\vspace{2mm}
\label{tab:inception_final_precision}
\centering
\begin{tabular}{lcccccccccccccc} \toprule
             &Block     &Layer(s)      &Layer Type    &Parameter Size(M)    & Weight bit   & Activation bit
             \\
    \midrule
             & Block 0  & Layer 0   & Conv         &    8.64e-4          &     6              & 6 \\
    \midrule
\gc             & Block 1  & Layer 1   & Conv         &    9.22e-3          &     6              & 6 \\
    \midrule
             & Block 2  & Layer 2   & Conv         &    1.84e-2          &     4              & 6 \\
    \midrule
\gc             & Block 3  & Layer 3   & Conv         &    5.12e-3          &     4              & 6 \\
    \midrule
             & Block 4  & Layer 4   & Conv         &    0.14             &     4              & 6 \\
    \midrule
\gc             & Block 5  & Layer 5-11   & Conv      &    0.25             &     4              & 4 \\
    \midrule
             & Block 6  & Layer 12-18  & Conv      &    0.28             &     4              & 4 \\
    \midrule
\gc             & Block 7  & Layer 19-25  & Conv      &    0.28             &     4              & 4 \\
    \midrule
             & Block 8  & Layer 26-29  & Conv      &    1.15             &     2              & 4 \\
    \midrule
\gc             & Block 9  & Layer 30-39  & Conv      &    1.29             &     4              & 4 \\
    \midrule
             & Block 10 & Layer 40-49  & Conv      &    1.69             &     4              & 4 \\
    \midrule
\gc             & Block 11 & Layer 50-59  & Conv      &    1.69             &     4              & 4 \\
    \midrule
             & Block 12 & Layer 60-69  & Conv      &    2.14             &     4              & 4 \\
    \midrule
\gc             & Block 13 & Layer 70-75  & Conv      &    1.70             &     2              & 4 \\
    \midrule
             & Block 14 & Layer 76-84  & Conv      &    5.04             &     2              & 4 \\
    \midrule
\gc             & Block 15 & Layer 85-93  & Conv      &    6.07             &     2              & 4 \\
    \midrule
             & Block 16 & Layer 94  & FC           &    2.05             &     2              & 4 \\
     \bottomrule

\end{tabular}
\end{table}
